# Supplementary material for: Relying on the Metrics of Evaluated Agents
Source: arXiv:2402.14005 source file (2024-10-28)
Supplement: Supplementary file 1 [file appendix_old.tex]

\begin{reptheorem}{thm:principal_not_worse}
Revealing $X$ always weakly increases the value of the principal ($\Vpr \geq \Vph$). Revealing $X$ strongly increases the value of the principal ($\Vpr > \Vph$) only if $X$ and $C$ are not independent. 
\end{reptheorem}
\begin{proof}
The solution $p_0 = p_1 = p$ is in the feasible set of the optimization problem with information revealed:
$$\max_{p_0, p_1} \;\; (1-\theta)F_0(p_0)(v - p_0) + \theta F_1(p_1)(v - p_1) $$
For this solution, the objective value is equal to $\Vph$; therefore, the maximum value of $\Vpr$ is at least the maximum value of $\Vph$.
If $X$ and $C$ are independent, or $F_0 = F_1 = F$, we have
$$\max_{p_0, p_1} \;\; (1-\theta)F(p_0)(v - p_0) + \theta F(p_1)(v - p_1) \leq \max_{p_0, p_1}\;\; (1-\theta)F(p_0)(v - p_0) + \max_{p_0, p_1} \;\; \theta F(p_1)(v - p_1) $$
The right hand side is the same as the maximum value of $\Vph$; therefore, the maximum value of $\Vpr$ is at most the maximum value of $\Vph$. We can also show this with first order conditions, which is more reminiscent of Holmstrom's sufficient statistic theorem.
\end{proof}

\begin{reptheorem}{thm:principal_value_increase}
Let $F_0$ and $F_1$ be continuously differentiable CDFs. Suppose $\Vpr$ is maximized by payments $p_0^{*}, p_1^{*}$ in the interior of the domain. If $F_0$ and $F_1$ satisfy $\frac{F_0(x)}{f_0(x)} < \frac{F_1(x)}{f_1(x)}$ for all $x$, then the principal strictly benefits when $X$ is revealed: $\Vpr > \Vph$.
\end{reptheorem}
\begin{proof}
Since $F_0$, $F_1$ are continuously differentiable and  $\Vpr$ is maximized by payments $p_0^{*}, p_1^{*}$ in the interior of the domain, the first order necessary conditions in Equation (\ref{eq:foc_x-revealed}) hold for the optimal payments $p_0^{*}$, $p_1^{*}$. By these first order necessary conditions, $p_0^{*} = p_1^{*}$ only if there exists a value $p$ such that 
$$p + \frac{F_0(p)}{f_0(p)} = p + \frac{F_1(p)}{f_1(p)} = v.$$
Such a value $p$ cannot exist if $\frac{F_0(p)}{f_0(p)} \neq \frac{F_1(p)}{f_1(p)}$ for all $p$. The MLRP implies that $\frac{F_0(p)}{f_0(p)} < \frac{F_1(p)}{f_1(p)}$ for all $p$; therefore, $p_0^{*} \neq p_1^{*}$, and maximum value for $\Vpr$ is strictly greater than the maximum value for $\Vph$.
\end{proof}

\begin{reptheorem}{thm:total_welfare_necessary}
Total welfare increases under revelation only if task completion quantity increases under revelation,
$$F(p^{*}) < (1-\theta)F_0(p_0^{*}) + \theta F_1(p_1^{*}).$$
\end{reptheorem}
\begin{proof}
\begin{align*}
    \Vjr - \Vjh &= (1-\theta) \int_{0}^{p_0^{*}}(v-c)f_0(c)dc + \theta \int_{0}^{p_1^{*}}(v-c)f_1(c)dc - \int_{0}^{p^{*}}(v-c) f(c)dc \\
    &= (1-\theta) \int_{0}^{p_0^{*}}(v-c)f_0(c)dc + \theta \int_{0}^{p_1^{*}}(v-c)f_1(c)dc \\
    &\quad - (1-\theta)\int_{0}^{p^{*}}(v-c)f_0(c)dc - \theta \int_{0}^{p^{*}}(v-c)f_1(c)dc \\
    &= (1-\theta) \int_{p^{*}}^{p_0^{*}}(v-c)f_0(c)dc - \theta \int_{p_1^{*}}^{p^{*}}(v-c)f_1(c)dc \\
\end{align*}

Upper bounding this:
\begin{align*}
    (1-\theta) \int_{p^{*}}^{p_0^{*}}(v-c)f_0(c)dc - \theta \int_{p_1^{*}}^{p^{*}}(v-c)f_1(c)dc &\leq (1-\theta) \int_{p^{*}}^{p_0^{*}}(v-p^{*})f_0(c)dc - \theta \int_{p_1^{*}}^{p^{*}}(v-p^{*})f_1(c)dc \\
    \implies \Vjr - \Vjh &\leq (v-p^{*}) \left((1-\theta) \int_{p^{*}}^{p_0^{*}}f_0(c)dc - \theta \int_{p_1^{*}}^{p^{*}}f_1(c)dc \right)
\end{align*}

The right hand term is exactly the difference in output:
\begin{align*}
    \left((1-\theta) \int_{p^{*}}^{p_0^{*}}f_0(c)dc - \theta \int_{p_1^{*}}^{p^{*}}f_1(c)dc \right) &= (1-\theta) (F_0(p_0^{*}) - F_0(p^{*})) - \theta (F_1(p^{*}) - F_1(p_1^{*})) \\
    &= (1-\theta)F_0(p_0^{*}) + \theta F_1(p_1^{*}) - ((1-\theta)F_0(p^{*}) + \theta F_1(p^{*})) \\
    &= (1-\theta)F_0(p_0^{*}) + \theta F_1(p_1^{*}) - F(p^{*}) \\
    \implies \Vjr - \Vjh &\leq (v-p^{*}) \left((1-\theta)F_0(p_0^{*}) + \theta F_1(p_1^{*}) - F(p^{*}) \right)
\end{align*}
Since $(v-p^{*}) > 0$, if output decreases,  $(1-\theta)F_0(p_0^{*}) + \theta F_1(p_1^{*}) - F(p^{*}) \leq 0$, then $\Vjr - \Vjh \leq 0$.
\end{proof}

\begin{reptheorem}{thm:total_welfare_sufficient}
Suppose $F_0$, $F_1$ are concave and satisfy the MLRP. Then total welfare increases under revelation if average output increases \textbf{by more than average cost} under revelation:

$$\frac{((1-\theta)F_0(p_0^{*}) + \theta F_1(p_1^{*}))}{F(p^{*})} > \frac{(v - g(p^{*}))}{(v - (1-\theta)(g_0(p_0^{*})) + \theta(g_1(p_1^{*}))} > 1,$$ 
where the functions $g$ represent the expected conditional cost:
$$g(p) = \frac{E[\Ind(C < p)C]}{F(p)},\;\; g_0(p_0) = \frac{E[\Ind(C < p_0)C | X = 0]}{F_0(p_0)},\;\; g_1(p_1) = \frac{E[\Ind(C < p_1)C | X = 1]}{F_1(p_1)}.$$
\end{reptheorem}
\begin{proof}
$$\Vjr - \Vjh = v((1-\theta)F_0(p_0^{*}) + \theta F_1(p_1^{*})- F(p^{*})) - ((1-\theta)F_0(p_0^{*})g_0(p_0^{*}) + \theta F_1(p_1^{*})g_1(p_1^{*}) - F(p^{*})g(p^{*}))  $$

If output increases under revelation, then the first term $v((1-\theta)F_0(p_0^{*}) + \theta F_1(p_1^{*})- F(p^{*}))$ is positive. 

% We now show that if output decreases under revelation, the second term is also positive: $$(1-\theta)F_0(p_0^{*})g_0(p_0^{*}) + \theta F_1(p_1^{*})g_1(p_1^{*}) > F(p^{*})g(p^{*}).$$ 

To bound the second term, Lemma \ref{lemma:split_costs} states that the expected conditional cost is higher in the higher-cost setting:
$$g_0(p_0^{*}) > g_1(p_1^{*}).$$

Then since $F_0(p_0^{*}) < F_1(p_1^{*})$, applying the identity from Lemma \ref{lemma:higher_averages},
\begin{align*}
    &(1-\theta) F_0(p_0^{*})(g_0(p_0^{*})) + \theta F_1(p_1^{*})(g_1(p_1^{*})) <  ((1-\theta)F_0(p_0^{*}) + \theta F_1(p_1^{*}))((1-\theta)(g_0(p_0^{*})) + \theta(g_1(p_1^{*})). \\
\end{align*}

Combining this with the first term: 
\begin{align*}
     \Vjr - \Vjh &= v((1-\theta)F_0(p_0^{*}) + \theta F_1(p_1^{*})- F(p^{*})) - ((1-\theta)F_0(p_0^{*})g_0(p_0^{*}) + \theta F_1(p_1^{*})g_1(p_1^{*}) - F(p^{*})g(p^{*})) \\
     &> (v - (1-\theta)(g_0(p_0^{*})) + \theta(g_1(p_1^{*}))((1-\theta)F_0(p_0^{*}) + \theta F_1(p_1^{*})) - (v - g(p^{*}))F(p^{*})
\end{align*}

% $$\Vjr - \Vjh > (v - (1-\theta)(g_0(p_0^{*})) + \theta(g_1(p_1^{*}))((1-\theta)F_0(p_0^{*}) + \theta F_1(p_1^{*})) - (v - g(p^{*}))F(p^{*})  $$

Lemma \ref{lemma:costs_increasing} states that the average conditional cost increases under revelation:
$$ (1-\theta)g_0(p_0^{*}) + \theta g_1(p_1^{*}) > g(p^{*}).$$
$$\implies v - ((1-\theta)(g_0(p_0^{*})) + \theta(g_1(p_1^{*})) < v-g(p^{*})$$

Thus, if output increases enough to outweight this difference,
$$\frac{((1-\theta)F_0(p_0^{*}) + \theta F_1(p_1^{*}))}{F(p^{*})} > \frac{(v - g(p^{*}))}{(v - (1-\theta)(g_0(p_0^{*})) + \theta(g_1(p_1^{*}))} > 1,$$ 

then $\Vjr - \Vjh > 0$ as well.
\end{proof}

\begin{lemma}\label{lemma:higher_averages}
(Covariance signs) $x_1 < x_2$ and $y_1 < y_2$ if and only if for any $\theta \in [0,1]$, 
$$(1-\theta)x_1y_1 + \theta x_2y_2 > ((1-\theta)x_1 + \theta y_1)((1-\theta)y_1 + \theta y_2).$$

\end{lemma}
\begin{proof}
For any $\theta \in [0,1]$,
\begin{align*}
    &(1-\theta)x_1y_1 + \theta x_2y_2 > ((1-\theta)x_1 + \theta x_2)((1-\theta)y_1 + \theta y_2) \\
    &\iff (1-\theta)x_1y_1 + \theta x_2y_2 > (1-\theta)^2 x_1y_1 + \theta^2 x_2y_2 + (1-\theta)\theta x_1y_2 +(1-\theta)\theta x_2y_1 \\
    &\iff ((1-\theta) - (1-\theta)^2) x_1y_1 + (\theta - \theta^2) x_2y_2 >  (1-\theta)\theta (x_1y_2 + x_2y_1) \\
    &\iff \frac{(1-\theta) - (1-\theta)^2}{(1-\theta)\theta} x_1y_1 + \frac{(\theta - \theta^2)}{(1-\theta)\theta} x_2y_2 >  x_1y_2 + x_2y_1 \\
    &\iff \frac{1 - (1-\theta)}{\theta} x_1y_1 + \frac{(1 - \theta)}{(1-\theta)} x_2y_2 >  x_1y_2 + x_2y_1 \\
    &\iff x_1y_1 + x_2y_2 >  x_1y_2 + x_2y_1 \\
    &\iff (x_1-x_2)(y_1-y_2) > 0 \\
    &\iff x_1 < x_2, y_1 < y_2
\end{align*}
\end{proof}

\begin{lemma}\label{lemma:split_costs}
If $F_0$, $F_1$ are concave and satisfy the MLRP, then
$$g_0(p_0^{*}) > g_1(p_1^{*}).$$

\end{lemma}
% \begin{proof}
% \snote{TODO}
% \end{proof}

\begin{lemma}\label{lemma:costs_increasing}
If $F_0$, $F_1$ are concave and satisfy the MLRP, then the expected costs are increasing under revelation: 
$$g(p^{*}) < (1-\theta)g_0(p_0^{*}) + \theta g_1(p_1^{*}).$$
\end{lemma}
% \begin{proof}
% \snote{TODO}
% \end{proof}


\section{Proofs from Section \ref{sec:garbling}}

We can rewrite $C | Y$ in terms of $C | X$ and $\veps$ as follows:
\begin{align*}
P(C = c | Y = 0)
&= \frac{(1-\theta)(1 + \veps)}{-2\theta\veps + \veps + 1} P(C = c | X = 0) + \frac{\theta(1-\veps)}{-2\theta\veps + \veps + 1}P(C = c | X = 1) \\
P(C = c | Y = 1)
&= \frac{\theta(1 + \veps)}{2\theta\veps - \veps + 1} P(C = c | X = 1) + \frac{(1-\theta)(1-\veps)}{2\theta\veps - \veps + 1}P(C = c | X = 0).
\end{align*}

When $\theta = \frac{1}{2}$, this simplifies to
\begin{align*}
P(C = c | Y = 0)
&= \frac{1 + \veps}{2} P(C = c | X = 0) + \frac{1 - \veps}{2}P(C = c | X = 1) \\
P(C = c | Y = 1)
&= \frac{1 + \veps}{2} P(C = c | X = 1) + \frac{1 - \veps}{2} P(C = c | X = 0).
\end{align*}

\begin{repproposition}{prop:garbling_principal} $\Vph \leq \Vpeps \leq \Vpr$ for all $\varepsilon$.
\end{repproposition}
\begin{proof}
    The proof for this follows directly from the principal's optimality conditions. Intuitively, if the principal receives a revealed signal, they can always recover any garbled solution by garbling the signal themselves.
\end{proof}

\begin{lemma}\label{lem:p_constant}
    Suppose that $f_0$ is bounded: $f_0(p) < B$ for all $p$ in the support $[0, \infty)$. Then for any fixed value $v$, there exists an $\delta$ such that for any $\veps > \delta$, $p_1^{\veps} = 0$. Furthermore, for $\veps > \delta$, there is no $p_1 > 0$ that would satisfy the first order condition,
    $$p_1 + \frac{\frac{1+\veps}{1-\veps} + F_0(p_1)}{f_0(p_1)} = v.$$
\end{lemma}
\begin{proof}
    Define $h(p, \veps) = p + \frac{1}{f_0(p)}\frac{1+\veps}{1-\veps} + \frac{F_0(p)}{f_0(p)}$. By choosing $\delta$ close to 1, we can make the term $\frac{1+\delta}{1-\delta}$ arbitrarily large, and consequently $\frac{1}{f_0(p_1)}\frac{1+\delta}{1-\delta}$ arbitrarily large, since $f_0(p) > 0$. Then for any $v$, we choose $\delta$ close enough to 1 such that $\frac{1}{B}\frac{1+\delta}{1-\delta} > v$. Since $p + \frac{F_0(p)}{f_0(p)} > 0$ for all $p$ in the support, there is no $p > 0$ that can satisfy the first order condition.
\end{proof}


\begin{reptheorem}{thm:garbling_zerocost}
    Suppose $\theta = \frac{1}{2}$, and suppose $C | X = 1$ takes value $0$ with probability 1 ($F_1(p) = 1$ for all $p > 0$). Then $\frac{\partial}{\partial \veps} \Vaeps |_{\veps = 1} < 0$ if and only if
    $$r(p_0^{*}) - r'(p_0^{*})g(p_0^{*}) - g(p_0^{*}) < 0,$$
    where $r(p) = \frac{F_0(p)}{f_0(p)}$ and $g(p) = \int_{0}^p (1-F_0(c))dc$.
\end{reptheorem}
\begin{proof}
\begin{align*}
    \frac{\partial}{\partial \veps} \Vaeps = &\frac{1}{2}\bigg(\frac{1 + \veps}{2}F_0(p_0^{\varepsilon})(\frac{\partial}{\partial \veps}p_0^{\varepsilon}) + \frac{1}{2}E[(p_0^{\varepsilon} - C)\Ind(C < p_0^{\varepsilon}) | X = 0] \\
    &\;\;+ \frac{1 - \veps}{2}(\frac{\partial}{\partial \veps}p_0^{\varepsilon}) - \frac{1}{2}p_0^{\veps}\bigg) \\
    + &\frac{1}{2}\bigg(\frac{1 + \veps}{2}(\frac{\partial}{\partial \veps}p_1^{\varepsilon}) + \frac{1}{2}p_1^{\varepsilon} \\
    &\;\;+ \frac{1 - \veps}{2}F_0(p_1^{\varepsilon})(\frac{\partial}{\partial \veps}p_1^{\varepsilon}) - \frac{1}{2}E[(p_1^{\varepsilon} - C) \Ind(C < p_1^{\varepsilon}) | X = 0]\bigg) 
\end{align*}
Evaluating at $\veps = 1$, by Lemma \ref{lem:p_constant}, $p_1^{\varepsilon}= 0$ and $\frac{\partial}{\partial \veps}p_1^{\varepsilon}|_{\veps = 1} = 0$.
Therefore,
\begin{align*}
    2\frac{\partial}{\partial \veps} \Vaeps |_{\veps = 1} = &F_0(p_0^{*})(\frac{\partial}{\partial \veps}p_0^{\varepsilon})|_{\veps = 1} + \frac{1}{2}E[(p_0^{*} - C)\Ind(C < p_0^{*}) | X = 0] - \frac{1}{2}p_0^{*}
\end{align*}
where 
$$\frac{\partial}{\partial \veps}p_0^{\varepsilon}|_{\veps = 1} = \frac{f_0(p_0^{*})}{4f_0(p_0^{*})^2 - 2F_0(p_0^{*})f_0'(p_0^{*})}$$

$$\implies 2\frac{\partial}{\partial \veps} \Vaeps |_{\veps = 1} = \frac{F_0(p_0^{*})f_0(p_0^{*})}{4f_0(p_0^{*})^2 - 2F_0(p_0^{*})f_0'(p_0^{*})} + \frac{1}{2}E[(p_0^{*} - C)\Ind(C < p_0^{*}) | X = 0] - \frac{1}{2}p_0^{*} $$

$$ 2\frac{\partial}{\partial \veps} \Vaeps |_{\veps = 1} < 0 \iff \frac{F_0(p_0^{*})}{f_0(p_0^{*})} - h'(p_0^{*})\left(\mu_0 - \int_{p_0^{*}}^{\infty} (c - p_0^{*})f_0(c)dc\right) < 0$$

$$g(p_0^{*}) = \mu_0 - \int_{p_0^{*}}^{\infty} (c - p_0^{*})f_0(c)dc$$
\end{proof}

% \section{Additional examples}

% \paragraph{Exponential distribution example.} To illustrate the implications of the hazard rate condition in Theorem \ref{thm:agent_value}, let $F_0\sim \text{Exp}(\lambda_0)$. Then the condition in \Eqref{eq:F0_condition} is equivalent to
% \begin{equation}\label{eq:exponential_lambda_bound}
%     \frac{\theta v}{\left(\left(\frac{1}{1-\theta}\right)^{\frac{1}{\theta}} - \left(\frac{1}{1-\theta}\right)^{\frac{1-\theta}{\theta}} - \theta \right)} >  \lambda_0.
% \end{equation}

% Thus, as long as the mean $\lambda_0$ is less than a threshold that depends on $\theta$ and $v$, the condition in Theorem \ref{thm:agent_value} holds. For any fixed $\theta$, this shows that if the higher cost setting $F_0$ is high enough, the agent will prefer to reveal. 

% Here we consider how this preference varies as a function of $\theta$, the probability of being in the zero-cost setting ($P(X = 1)$). Figure \ref{fig:exponential_lambda_bound} illustrates this bound on $\lambda_0$ as a function of $\theta$. For higher values of $\theta$, the curve shows that when the agent has a high chance of incurring zero cost, $\lambda_0$ does not have to be very high for revelation to help the agent. On the other hand, if the agent has a low chance of incurring zero cost, then the agent would be more likely to prefer to keep their information hidden.

% \begin{figure}[!ht]
%     \centering
%     \includegraphics[width=0.4\textwidth]{figures/exponential_lambda_bound.png}
%     \caption{Graph of the inequality in \Eqref{eq:exponential_lambda_bound} for $v = 1$, where $g(\theta,v) = \frac{\theta v}{\left(\left(\frac{1}{1-\theta}\right)^{\frac{1}{\theta}} - \left(\frac{1}{1-\theta}\right)^{\frac{1-\theta}{\theta}} - \theta \right)}$, and $\lambda_0 < g(\theta,v)$ is the set of $\lambda_0$ values that trigger Theorem \ref{thm:agent_value}. For any fixed $\theta$, if $\lambda_0$ is below the threshold $g(\theta, v)$, then the agent will prefer to keep their information hidden. As the probability of being in the zero-cost setting $\theta$ increases, that threshold also decreases, meaning that the $\lambda_0$ required to make the agent want to reveal gets lower. }
%     \label{fig:exponential_lambda_bound}
% \end{figure}
